# Supplementary material for: SynKB: Semantic Search for Synthetic Procedures
Source: arXiv:2208.07400 source file (2022-10-06)
Supplement: Supplementary file 1 [file appendix.tex]

\begin{table*}[th!]
\small
\centering
\scalebox{0.9}{
\begin{tabular}{c|L{14cm}}
\toprule 
\tabf{\textbf{System}} & \tabf{\textbf{Q1} - What are the \textbf{solvents} used for reactions containing the reagent \textbf{triphosgene}?} \\ \midrule

 \tabf{\multirow{2}{*}[-0.8em]{\reaxys{}}}  & \tabf{{\it \textbf{Triphosgene} (79.4 mg, 0.268 mmol) was dissolved in 1.5 mL of \sethlcolor{lightblue}\textbf{\textcolor{blue}{\hl{dichloromethane}}}.}} \\
 \cmidrule{2-2}
 
& \tabf{{\it ... the instillment contains 89g (0.3mol) toluene solution of \textbf{triphosgene}... After the reaction, dropping 282.5g (2.0mol) boron trifluoride \sethlcolor{lightblue}\textbf{\textcolor{blue}{\hl{tetrahydrofuran}}} solution.}} \\ \midrule

%  \tabf{\multirow{2}{*}[-0.8em]{\synkb{}}}  & \tabf{{\it \textbf{Triphosgene} (90 mg) was added to a solution of the intermediate and triethylamine (0.027 ml) in \sethlcolor{lightblue}\textbf{\textcolor{blue}{\hl{chloroform}}} (1 ml) at 0 °C.}} \\ 
%  \cmidrule{2-2}
 
 \tabf{\multirow{2}{*}[-1em]{\synkb{}}} & \tabf{{\it ... in the presence of N,N-carbonyldiimidazole, phosgene or \textbf{triphosgene} ... The above reactions are conducted in an inert solvent, such as, ... , \sethlcolor{lightblue}\textbf{\textcolor{blue}{\hl{N,N-dimethylformamide}}}, dimethyl \sethlcolor{lightgrey}\textcolor{darkgrey}{\textbf{\hl{sulfoxide}}} and so on ...}} \\
  \cmidrule{2-2}
 
 & \tabf{{\it To a solution of (4S)-7-(2-methylp..., was added \textbf{triphosgene} (353 mg, 1.189 mmol) at 0 °C. ... \sethlcolor{pink}\textbf{\textcolor{darkred}{\hl{N-ethyl-N-isopropylpropan-2-amine}}} (307 mg, 2.378 mmol) were added at 27 ° C.}} \\ 
 \midrule
 \midrule
 
 & \tabf{\textbf{Q5} - What are the \textbf{reaction times} for reactions using \textbf{CDI (carbonyldiimidazole)}?} \\ \midrule

 \tabf{\multirow{2}{*}[-0.8em]{\reaxys{}}}  & \tabf{{\it To a room-temperature (RT) solution of \textbf{carbonyl diimidazole (CDI)}... The reaction mixture was stirred for \sethlcolor{lightblue}\textbf{\textcolor{blue}{\hl{10 min}}}... The reaction mixture was stirred another \sethlcolor{lightyellow}\textbf{\textcolor{darkyellow}{\hl{0.5-2 hour}}}.}} \\ 
 \cmidrule{2-2}
 
 & \tabf{{\it A solution of ... was treated with \textbf{CDI} (97 mg, 0.60 mmol) and stirred for \sethlcolor{lightblue}\textbf{\textcolor{blue}{\hl{15min}}}. ... the reaction mixture heated in a microwave at 180C for \sethlcolor{lightblue}\textbf{\textcolor{blue}{\hl{20mins}}}. The reaction mixture ..., eluting ... over \sethlcolor{lightyellow}\textbf{\textcolor{darkyellow}{\hl{9mins}}}...}} \\ \midrule
 
 \tabf{\multirow{2}{*}[-1em]{\synkb{}}}   & \tabf{{\it \textbf{Carbonyldiimidazole} (0.46 g, 2.8 retool) was added to a stirred solution ... After \sethlcolor{lightblue}\textbf{\textcolor{blue}{\hl{5 minutes}}}, the solvent was removed and the residue was dissolved...}} \\ 
 \cmidrule{2-2}
 
& \tabf{{\it A mixture of 7.2 g of the compound obtained in step B and 6.7 g of \textbf{1,1'-carbonyldiimidazole} in 100 ml of acetonitrile is refluxed for \sethlcolor{lightblue}\textbf{\textcolor{blue}{\hl{5 minutes}}}...}} \\ 
% \midrule
% \midrule

% & \tabf{\textbf{Q3} - What \textbf{molar concentration} is the reagent \textbf{HATU} at when \textbf{dissolved} in the solvent \textbf{DMF}?} \\ \midrule

%  \tabf{\multirow{2}{*}[-0.3em]{\synkb{}}}  & \tabf{{\it ... DIPEA (4 ml, 22.89 mmol) and \textbf{HATU} (3.05 g, \sethlcolor{lightblue}\textbf{\textcolor{blue}{\hl{8.02 mmol}}}) were dissolved in \textbf{DMF} (\sethlcolor{lightblue}\textbf{\textcolor{blue}{\hl{20 ml}}}) and stirred at room temperature for 15 mins...}} \\ 
% \cmidrule{2-2}

% & \tabf{{\it ... Diisopropylethylamine (0.836 ml, 4.8 mmol) was added to the reaction mixture and stirred at room temperature. In a separate flask, \textbf{HATU}, (670 mg, \sethlcolor{lightblue}\textbf{\textcolor{blue}{\hl{1.8 mmol}}}) was dissolved in anhydrous \textbf{DMF} (\sethlcolor{lightblue}\textbf{\textcolor{blue}{\hl{2 ml}}})...}} \\ 
 \bottomrule
\end{tabular}
}
\caption{\label{tab:sampled_output} Samples of results returned by \synkb{} (ours) and \reaxys{}. We use different colors to mark different types of results: \sethlcolor{lightblue}\textbf{\textcolor{blue}{\hl{correct answers}}}, \sethlcolor{pink}\textbf{\textcolor{darkred}{\hl{classification errors}}}, \sethlcolor{lightyellow}\textbf{\textcolor{darkyellow}{\hl{missing errors}}}, and \sethlcolor{lightgrey}\textcolor{darkgrey}{\textbf{\hl{segmentation errors}}}. \synkb{} has good coverage and high precision on entity classification and segmentation, while \reaxys{} has high precision, but lower recall, e.g., in Q2, it fails to capture all reaction times in the same procedure.
}
\end{table*}
